# Supplementary material for: Adjoint-based machine learning for active flow control
Source: arXiv:2307.09980 source file (2023-07-19)
Supplement: Supplementary file 1 [file 07_appendix.tex]

\section{Appendix}

\subsection{DPM vs DRL without Critic ANN} \label{sec:noCritic} 
% \begin{figure}[H]
%     \centering
%     \includegraphics[height=6.0cm]{Figures/FEniCS/Compare/ControlPerformance/noCritic/Cl_cmp.pdf}
%     \caption{Control performance of DPM and DRL comparison with different ANN complexity}
%     \label{fig:complexity}
% \end{figure}
The DRL models without the critic NN control performance are investigated here. There are 4 DRL actuators with different ANN complexity, where 2.6k and 19.4k parm/pt are trained with critic ANN, and 1.3k and 9.7k parm/pt are trained without critic ANN. The more complicated one in both groups utilizes two-layer NNs and the other one utilizes one-layer NNs.

Non-dimensional time series of the lift coefficient $C_l$, drag coefficient $C_d$, and statistical measures (on the second half simulation) of controlled flow based on DPM and DRL regulators compared with the baseline simulation (i.e. no active control).  It is clear that the existence of a critic network is critical to the effectiveness of drag reduction. Because it allows the agent to learn a more accurate estimate of the value of actions and states in PPO, which leads to more effective decision-making and better overall performance.

% Two phases can be observed in the flow configuration with a successive control transition from $t=0$ to $0.6$.
% The drag reduction of the DPM controller and the 19.4k parm/pt DRL controller around 26.7\% and 5.5\% are observed. The flow oscillation is 100\% compressed approximately to a steady state utilizing the DPM actuator, while the DRL controller is one and two orders of magnitude less effective. The control performance of all other DRL models enen with two hidden layers (i.e. 9.7k parm/pt) can be ignored.

\begin{figure}[H]
    \centering
    \includegraphics[width=1.0\linewidth]{Figures/FEniCS/Compare/ControlPerformance/noCritic.pdf}
    \caption{ Non-dimensional time series of the drag coefficient and statistical measures (on the second half simulation) of flows controlled by DRL actuators with and without critic NN, DPM actuator, and the uncontrolled baseline flow. There are 4 DRL models with different ANN complexity, 2.6k and 19.4k parm/pt are trained with  critic ANN and 1.3k and 9.7k parm/pt are trained without critic ANN.}
    \label{fig:complexityAppx}
\end{figure}
